# Supplementary material for: Synthesizing Speech from Intracranial Depth Electrodes using an Encoder-Decoder Framework
Source: arXiv:2111.01457 source file (2022-10-31)
Supplement: Supplementary file 1 [file appendix.tex]

\begin{figure}[h]
\centering
\begin{tabular}{lll}

\includegraphics[width=0.355\textwidth]{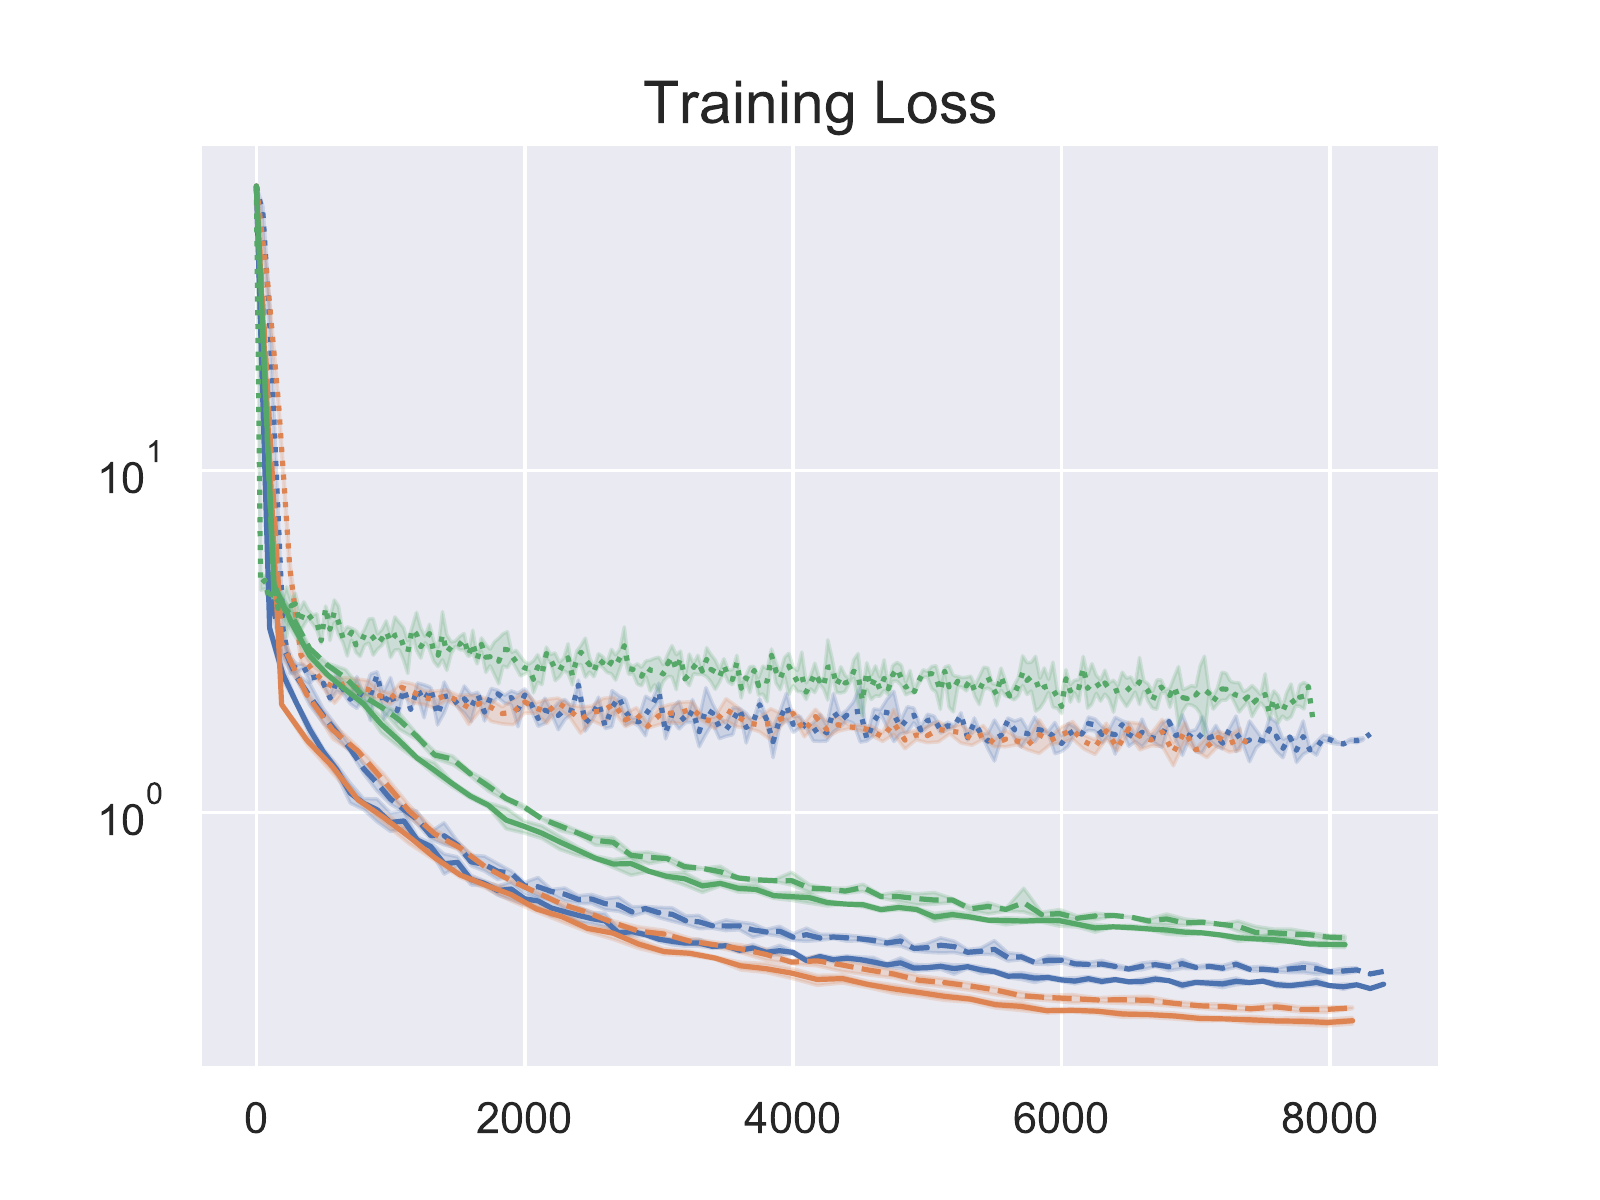}& \hspace{-0.75cm}
\includegraphics[width=0.355\textwidth]{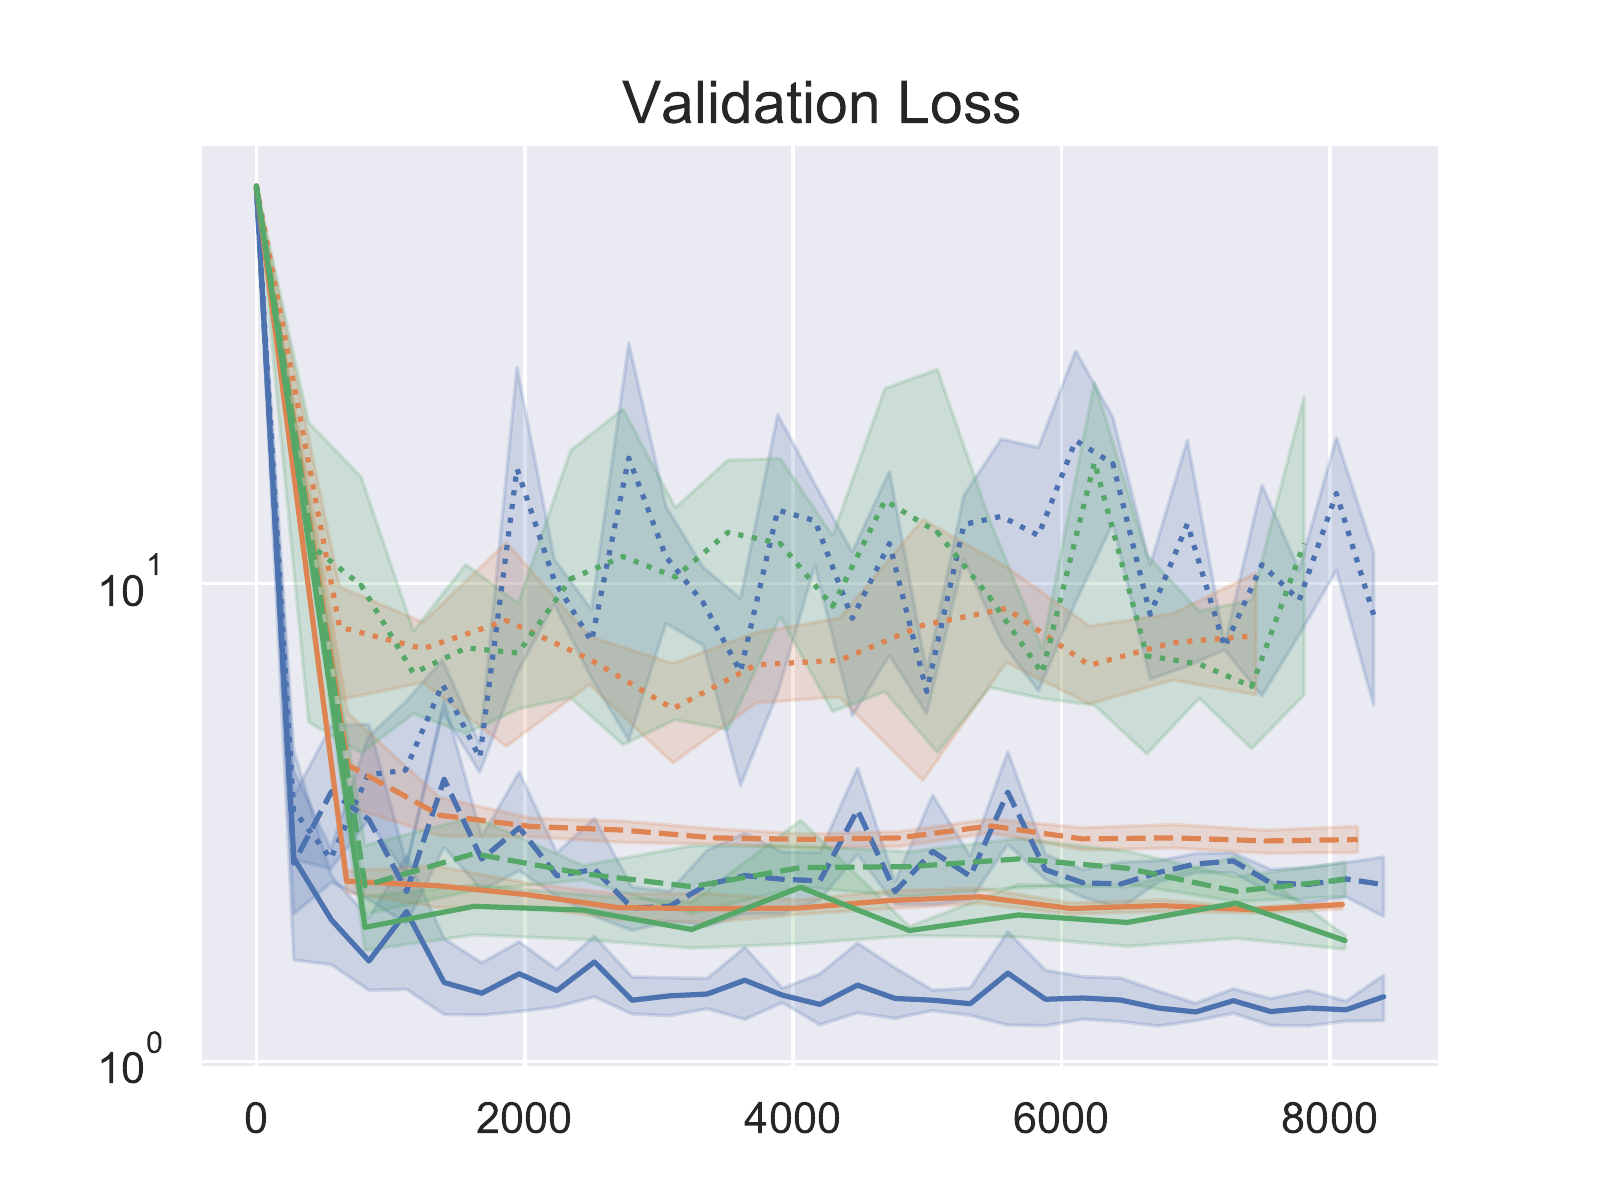}&\hspace{-0.75cm}
\includegraphics[width=0.355\textwidth]{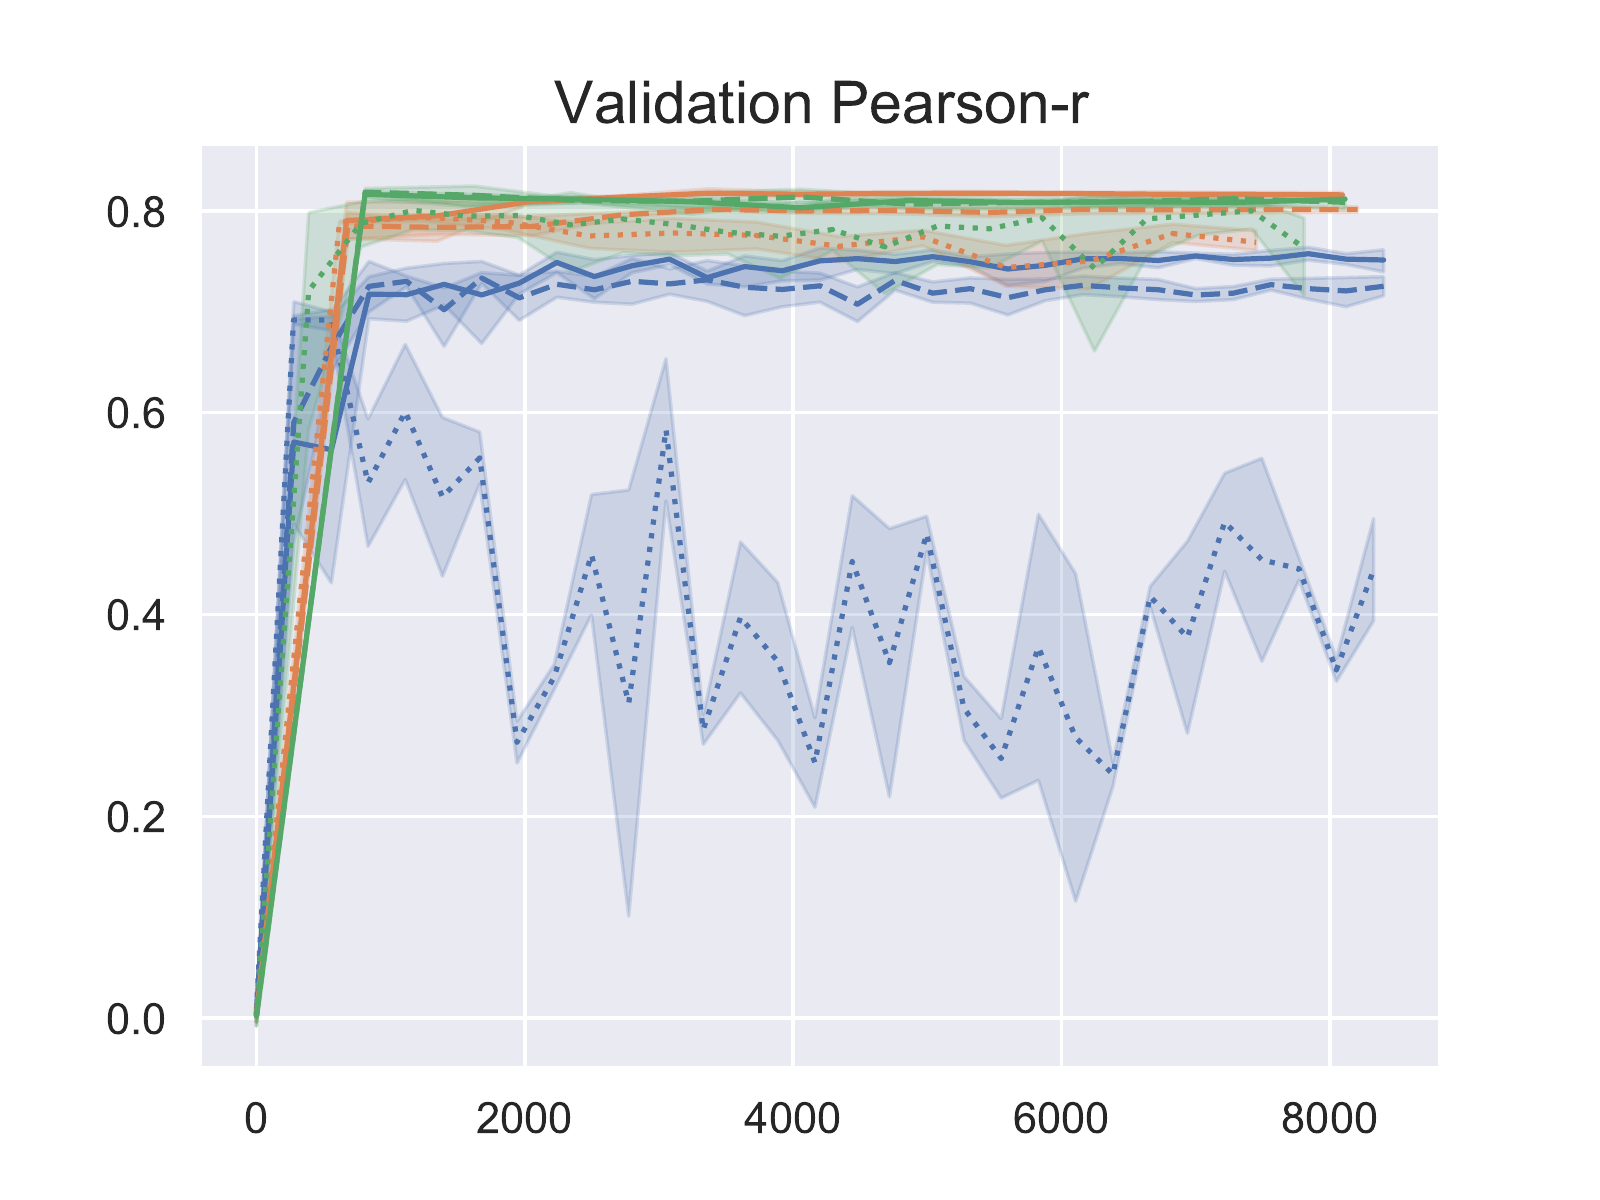}\\

\multicolumn{3}{c}{
\includegraphics[width=.66\textwidth]{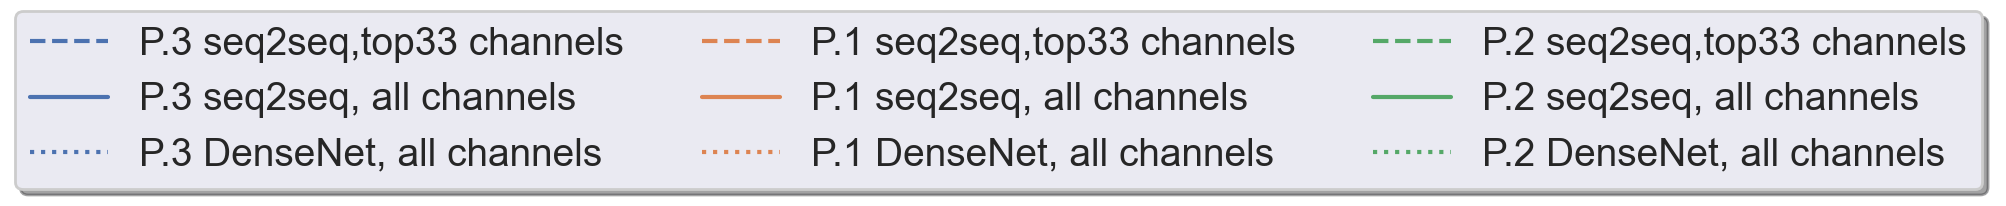}}

\end{tabular}

\caption{ \textbf{Training curves} Train and validation loss (log-scale) as well as Pearson correlation coefficient on validation set. Average and $95\%$ confidence interval over 5 independent runs.}

\vspace{-3mm}

\label{fig:train_curves}
\end{figure}

\begin{figure}[h]
\vspace{0.5cm}
\includegraphics[width=.99\textwidth]{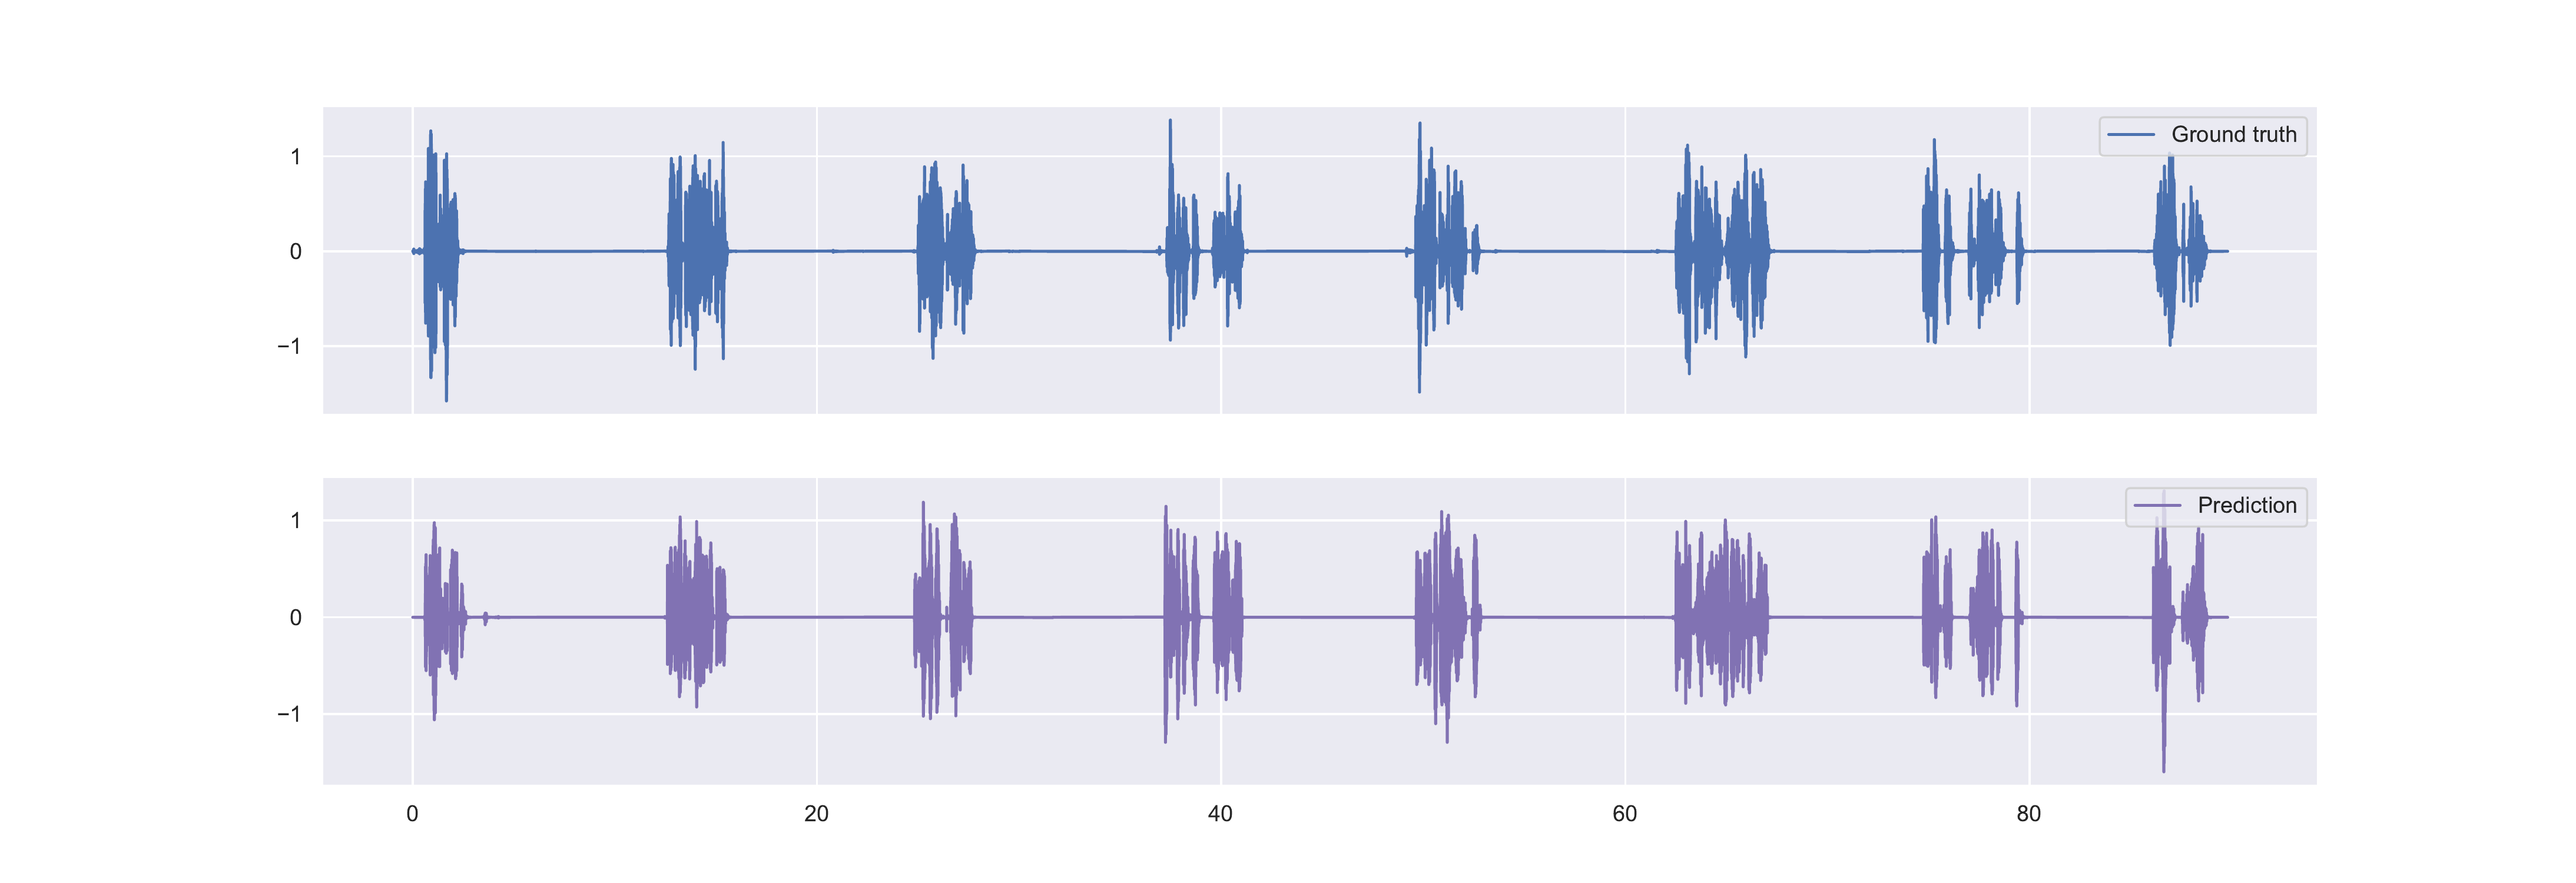}\hfill\\
\caption{ \textbf{Patient 3:} Waveforms of entire validation set: targets are in the first- and predictions in bottom row.}
\label{fig:p3_waves}
\end{figure}

\begin{figure}[h]
\vspace{0.5cm}
\includegraphics[width=.99\textwidth]{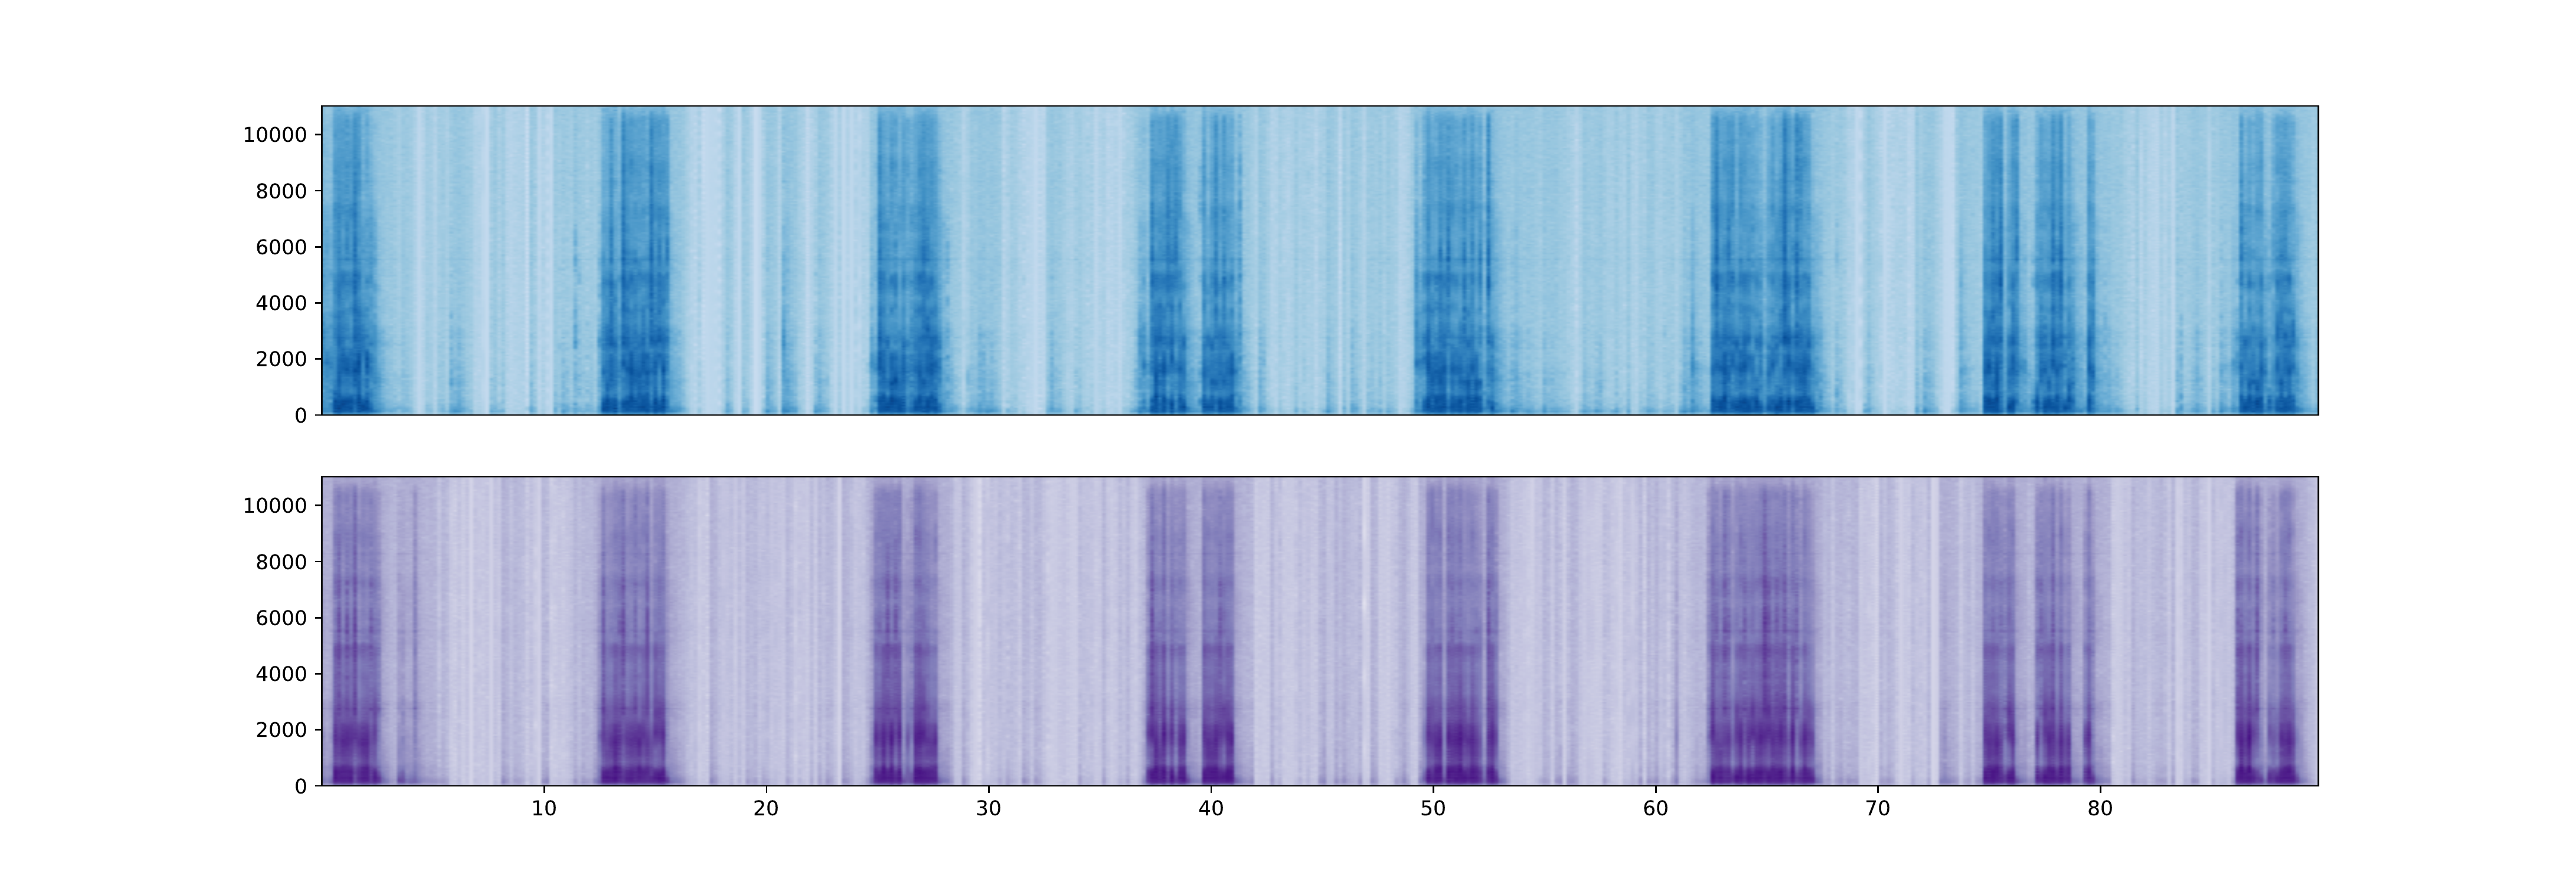}\hfill\\
\caption{ \textbf{Patient 3:} Spectograms of entire validation set: targets are in the first- and predictions in bottom row.}
\label{fig:p3_spec}
\end{figure}
